# Supplementary material for: Vacancy-induced low-energy states in undoped graphene
Source: arXiv:1602.09085 source file (2016-06-10)
Supplement: Supplementary file 1 [file scaling_plots_6p25.tex]

\documentclass[notitlepage]{report}
\usepackage[nohead, nomarginpar, margin=1in, foot=0in]{geometry}
\makeatletter
\setlength{\@fptop}{0pt}
\makeatother
\usepackage{subfig}
\usepackage{graphicx}

\date{}
\begin{document}

\begin{figure} 
\centerline{\includegraphics[width=0.3\columnwidth]{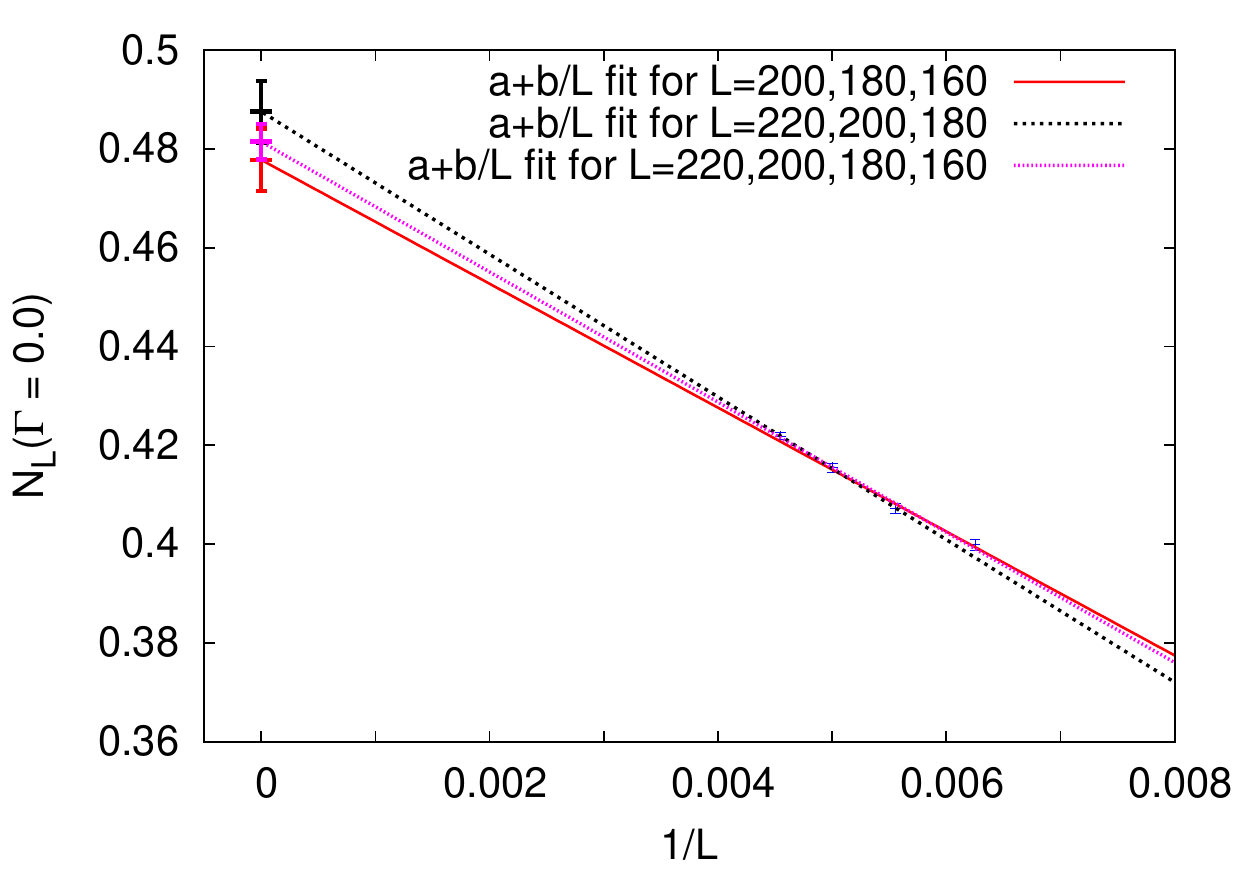}~
\includegraphics[width=0.3\columnwidth]{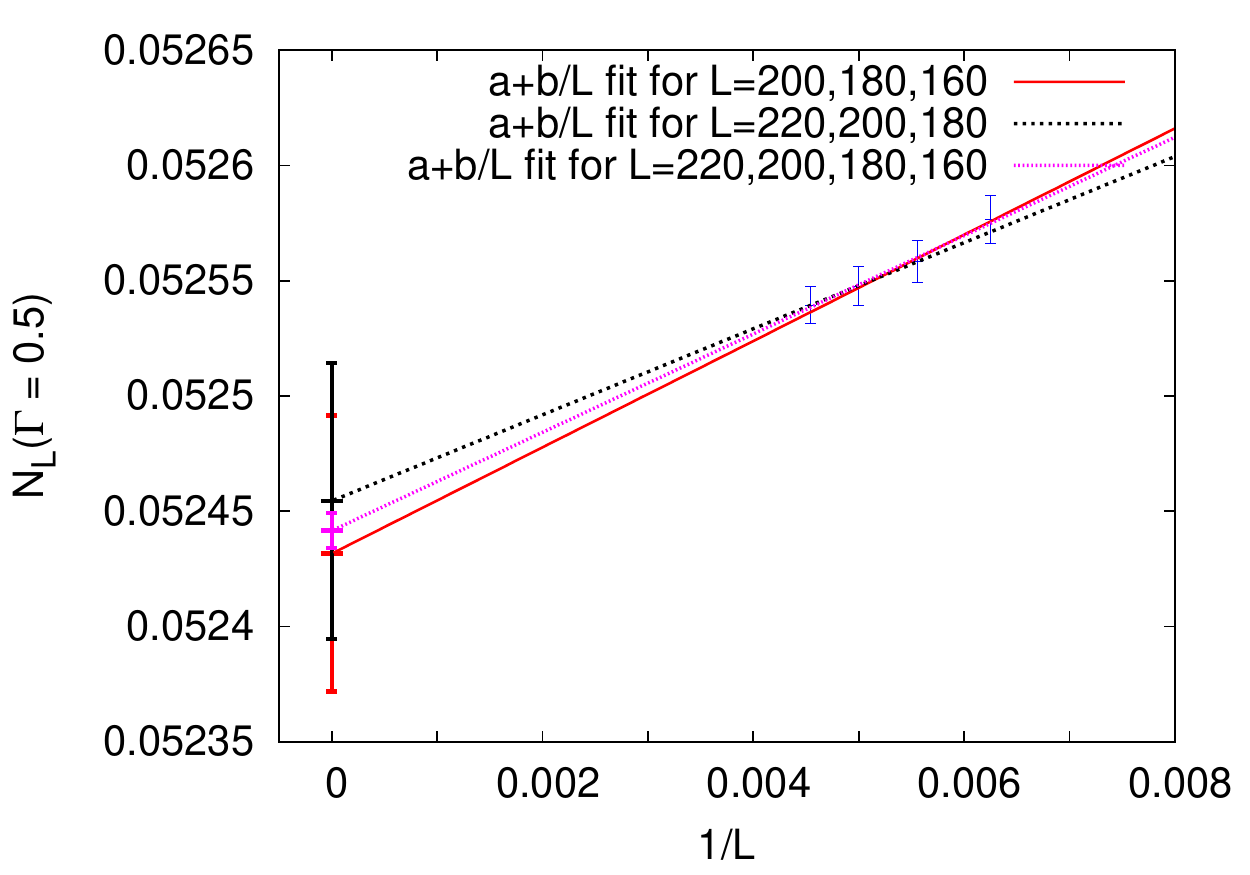}~
\includegraphics[width=0.3\columnwidth]{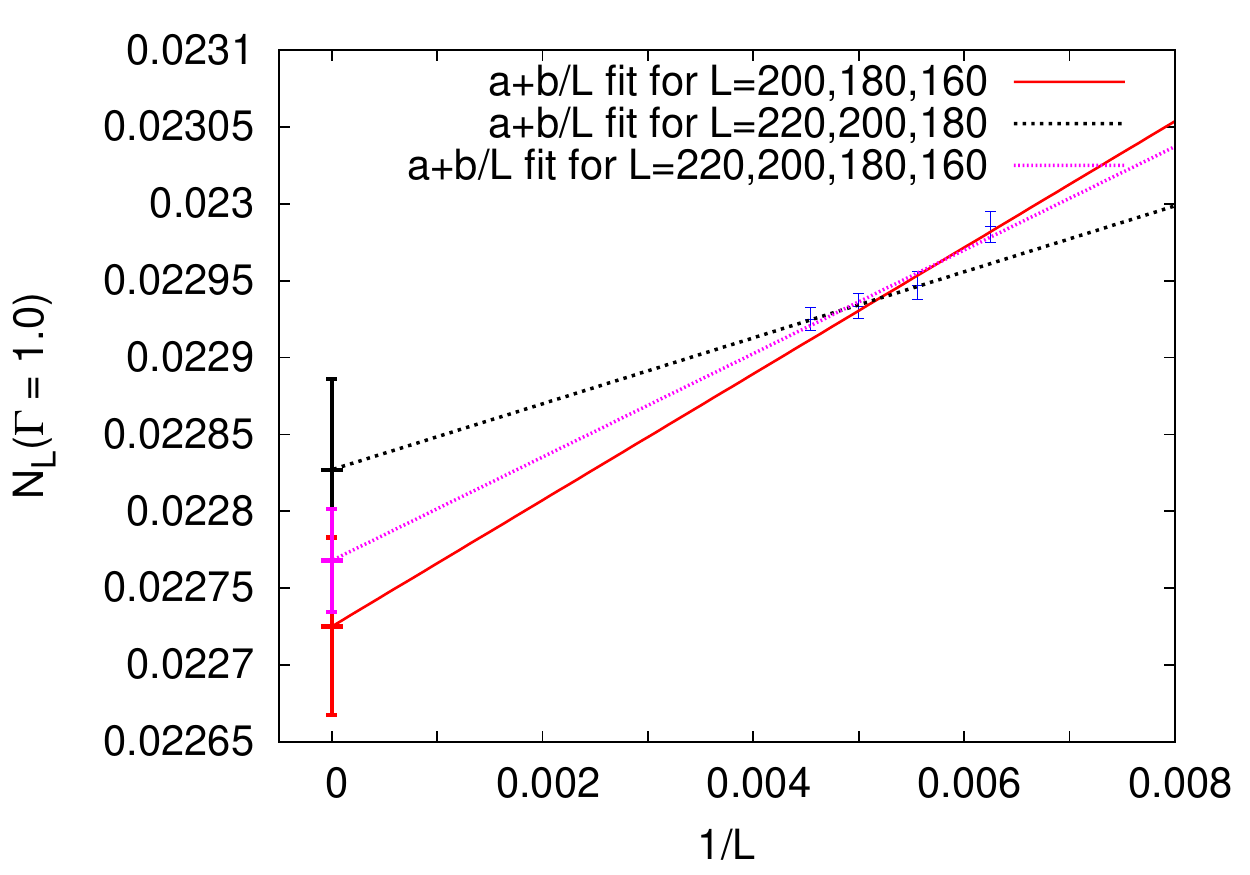}}
\centerline{\includegraphics[width=0.3\columnwidth]{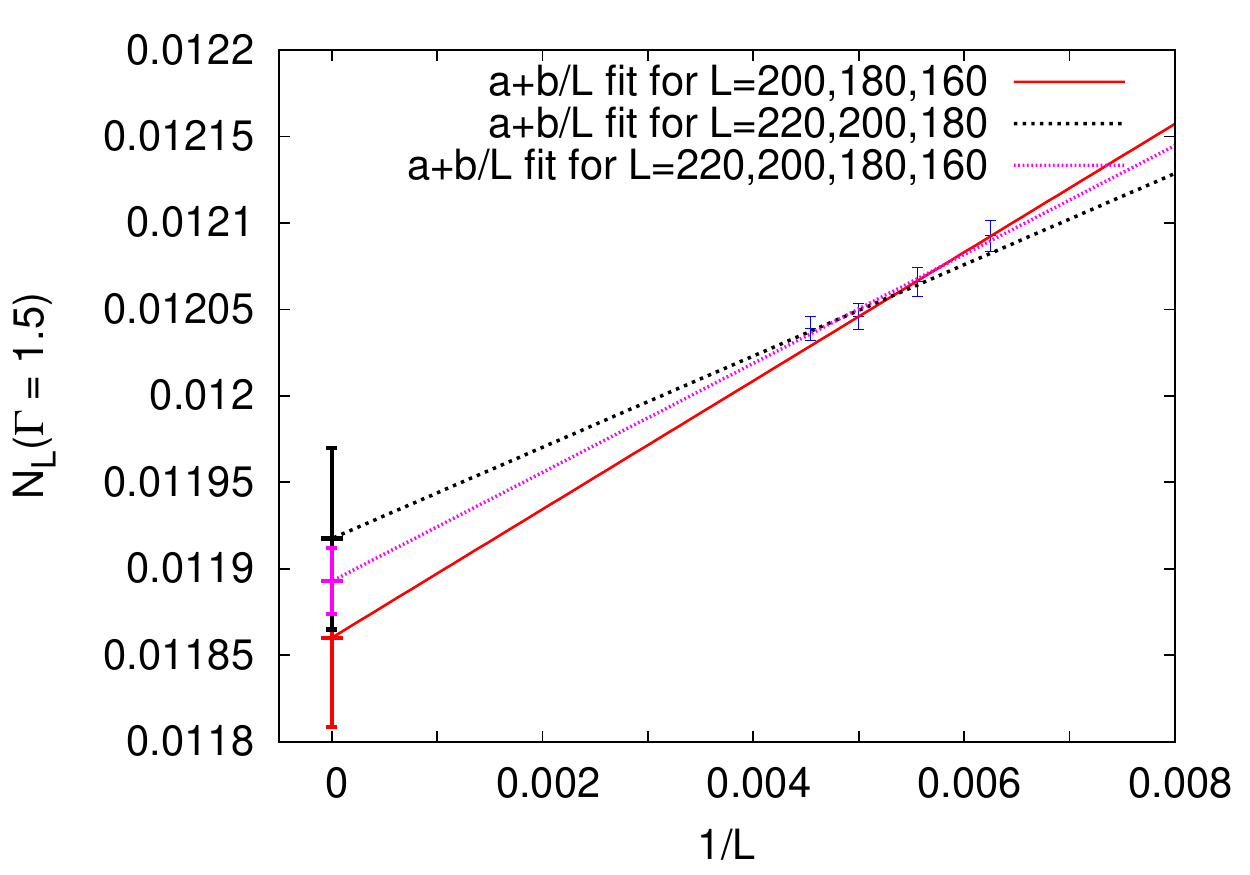}~
\includegraphics[width=0.3\columnwidth]{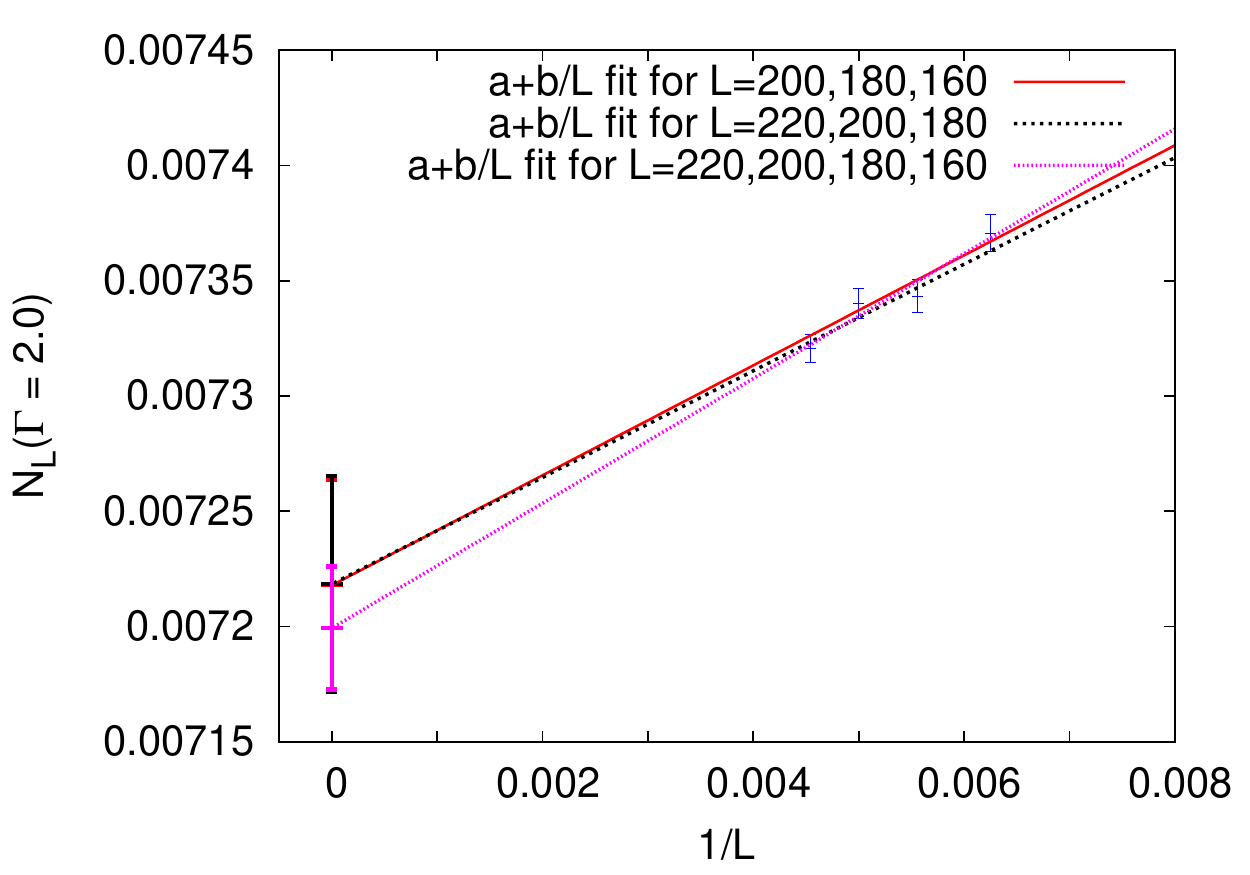}~
\includegraphics[width=0.3\columnwidth]{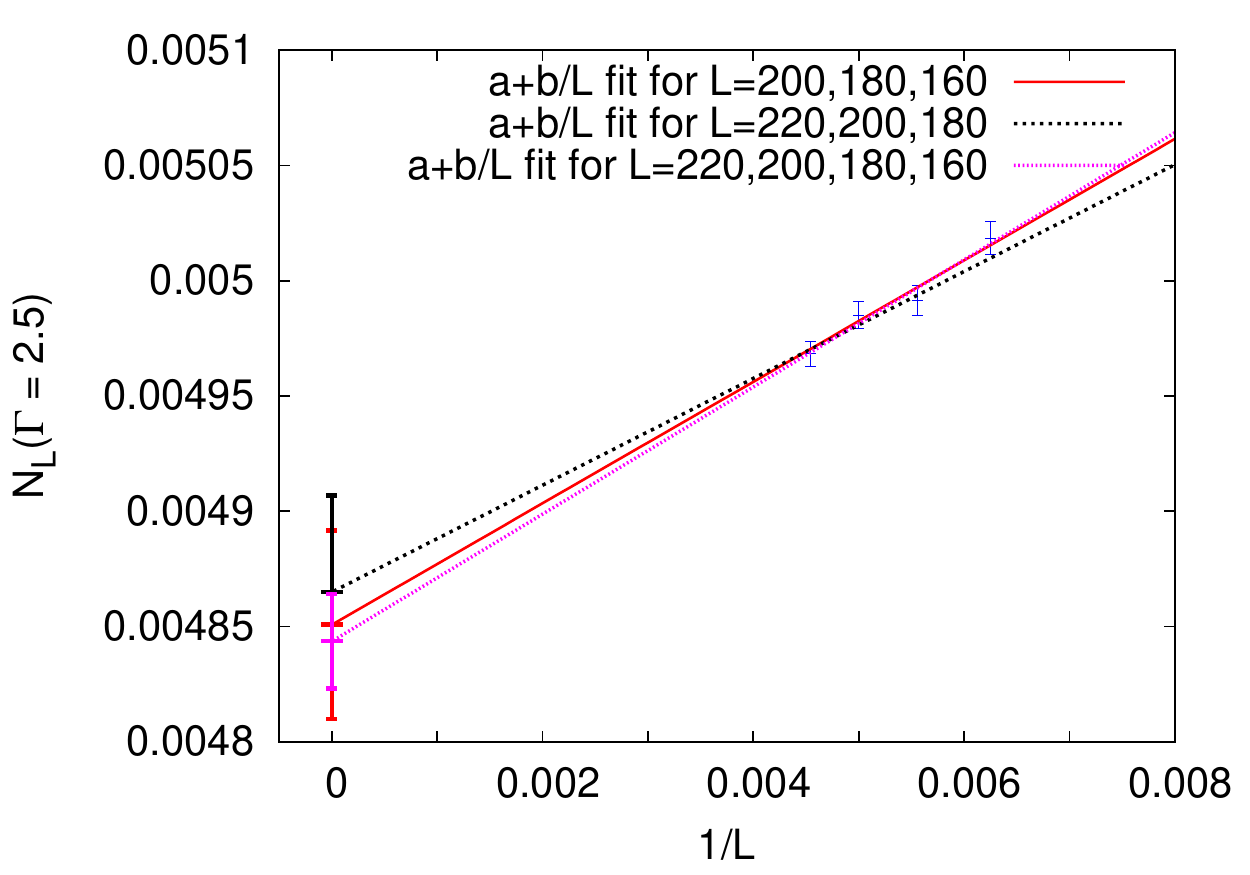}}
\caption { 
\label{fig:PhaseDiagram}}
\end{figure}

\end{document}
